# Supplementary material for: Universal effective couplings of the three-dimensional $n$-vector model and field theory
Source: arXiv:1909.05823 ancillary file (2020-01-21)
Supplement: Supplementary file 1 [file rg_expansions_couplings_g8_g10.pdf]

# Universal effective couplings of the three-dimensional $n$ -vector model and field theory

A. Kudlis<sup>a,\*</sup>, A. I. Sokolov<sup>a</sup>

<sup>a</sup>*St. Petersburg State University, 7/9 Universitetskaya Emb., St. Petersburg, 199034 Russia*

---

## Abstract

This document contains Tables with coefficients of RG expansions for  $g_8$  and  $g_{10}$  in four- and three-loop approximation respectively.

*Keywords:* renormalization group, multi-loop calculations, effective coupling constants, universal ratios.

*2000 MSC:* 82B28

---

## 1. Tables

Table 1: Feynman graphs for effective coupling  $g_8$

| No.                    | Graph description,<br>Nickel's notations | Integral value $\times (8\pi)^L$ ,<br>$L$ – number of loops | Symmetry<br>factor | Tensor factor $\times 3^{L+3}$ ,<br>$L$ – number of loops |
|------------------------|------------------------------------------|-------------------------------------------------------------|--------------------|-----------------------------------------------------------|
| 1-1                    | $ee12 ee3 ee3 ee $                       | 1/8                                                         | 315                | $80 + n$                                                  |
| 2-1                    | $ee11 23 ee4 ee4 ee $                    | 1/8                                                         | 630                | $212 + 30n + n^2$                                         |
| 2-2                    | $ee12 ee2 34 ee4 ee $                    | 1/16                                                        | 315                | $224 + 18n + n^2$                                         |
| 2-3                    | $ee12 ee3 ee4 e44 e $                    | 19/162                                                      | 1260               | $214 + 29n$                                               |
| 2-4                    | $ee12 ee3 e34 e4 ee $                    | 5/108                                                       | 2520               | $230 + 13n$                                               |
| 2-5                    | $ee12 e34 e34 ee ee $                    | 1/27                                                        | 420                | $234 + 9n$                                                |
| 3-1                    | $ee11 22 34 ee5 ee5 ee $                 | 1/8                                                         | 315                | $528 + 168n + 32n^2 + n^3$                                |
| 3-2                    | $ee11 23 ee3 45 ee5 ee $                 | 1/16                                                        | 630                | $584 + 128n + 16n^2 + n^3$                                |
| 3-3                    | $ee11 23 ee4 ee4 55 ee $                 | 1/8                                                         | 157.5              | $560 + 152n + 16n^2 + n^3$                                |
| 3-4                    | $ee11 23 ee4 ee5 e55 e $                 | 19/162                                                      | 630                | $568 + 150n + 11n^2$                                      |
| Continued on next page |                                          |                                                             |                    |                                                           |

---

\*Corresponding author

Email address: andrewkudlis@gmail.com (A. Kudlis)

Table 1 Feynman graphs for effective coupling  $g_8$ 

| No.  | Graph description,<br>Nickel's notations | Integral value $\times (8\pi)^L$ ,<br>$L$ – number of loops | Symmetry<br>factor | Tensor factor $\times 3^{L+3}$ ,<br>$L$ – number of loops |
|------|------------------------------------------|-------------------------------------------------------------|--------------------|-----------------------------------------------------------|
| 3-5  | $ee11 23 ee4 e45 e5 ee $                 | 5/108                                                       | 2520               | $608 + 114n + 7n^2$                                       |
| 3-6  | $ee11 23 ee4 e55 ee5 e $                 | 19/162                                                      | 1260               | $568 + 150n + 11n^2$                                      |
| 3-7  | $ee11 23 ee4 455 ee ee $                 | 1/8                                                         | 315                | $560 + 152n + 16n^2 + n^3$                                |
| 3-8  | $ee11 23 e34 e5 ee5 ee $                 | 5/108                                                       | 1260               | $600 + 118n + 11n^2$                                      |
| 3-9  | $ee11 23 e45 e45 ee ee $                 | 1/27                                                        | 630                | $616 + 106n + 7n^2$                                       |
| 3-10 | $ee12 ee2 33 45 ee5 ee $                 | 1/16                                                        | 157.5              | $576 + 132n + 20n^2 + n^3$                                |
| 3-11 | $ee12 ee2 34 ee5 e55 e $                 | 1/18                                                        | 1260               | $604 + 120n + 5n^2$                                       |
| 3-12 | $ee12 ee2 34 e45 e5 ee $                 | 1/36                                                        | 1260               | $636 + 88n + 5n^2$                                        |
| 3-13 | $ee12 ee3 ee3 45 e55 e $                 | 1/12                                                        | 630                | $584 + 142n + 3n^2$                                       |
| 3-14 | $ee12 ee3 ee4 ee5 555  $                 | $415/4608 - 5/16 \log[4/3]$                                 | 210                | $480 + 246n + 3n^2$                                       |
| 3-15 | $ee12 ee3 ee4 e45 55 e $                 | $-71/864 + 89 \log[4/3]/162$                                | 2520               | $588 + 140n + n^2$                                        |
| 3-16 | $ee12 ee3 ee4 e55 e55  $                 | 0.110545898524682                                           | 630                | $536 + 166n + 27n^2$                                      |
| 3-17 | $ee12 ee3 ee4 445 5 ee $                 | 31/384                                                      | 630                | $584 + 142n + 3n^2$                                       |
| 3-18 | $ee12 ee3 e34 e5 e55 e $                 | $17/108 - 11 \log[4/3]/27$                                  | 2520               | $620 + 108n + n^2$                                        |
| 3-19 | $ee12 ee3 e34 45 e5 ee $                 | 19/864                                                      | 5040               | $652 + 76n + n^2$                                         |
| 3-20 | $ee12 ee3 e34 55 ee5 e $                 | $17/108 - 11 \log[4/3]/27$                                  | 2520               | $616 + 110n + 3n^2$                                       |
| 3-21 | $ee12 ee3 e44 e45 5 ee $                 | $4 \log[4/3]/27$                                            | 2520               | $604 + 116n + 9n^2$                                       |
| 3-22 | $ee12 ee3 e44 e55 e5 e $                 | 0.110545898524682                                           | 1260               | $572 + 148n + 9n^2$                                       |
| 3-23 | $ee12 ee3 e45 e45 e5 e $                 | 0.019439866320025                                           | 2520               | $658 + 71n$                                               |
| 3-24 | $ee12 ee3 e45 445 e ee $                 | $-47/288 + 19 \log[4/3]/27$                                 | 2520               | $620 + 108n + n^2$                                        |
| 3-25 | $ee12 ee3 334 5 ee5 ee $                 | 13/256                                                      | 315                | $608 + 118n + 3n^2$                                       |
| 3-26 | $ee12 ee3 345 45 ee ee $                 | 3/128                                                       | 630                | $648 + 78n + 3n^2$                                        |
| 3-27 | $ee12 e23 e4 ee5 e55 e $                 | $4 \log[4/3]/27$                                            | 5040               | $616 + 110n + 3n^2$                                       |
| 3-28 | $ee12 e23 e4 e45 e5 ee $                 | 1/54                                                        | 2520               | $660 + 68n + n^2$                                         |
| 3-29 | $ee12 e23 45 ee4 e5 ee $                 | 1/54                                                        | 2520               | $656 + 70n + 3n^2$                                        |
| 3-30 | $ee12 e23 45 e45 ee ee $                 | 7/432                                                       | 2520               | $668 + 60n + n^2$                                         |
| 3-31 | $ee12 e33 e44 e5 e5 ee $                 | 0.110545898524682                                           | 630                | $572 + 148n + 9n^2$                                       |
| 3-32 | $ee12 e33 e45 45 ee ee $                 | $11/54 - 16 \log[4/3]/27$                                   | 1260               | $624 + 102n + 3n^2$                                       |
| 3-33 | $ee12 e34 e34 e5 e5 ee $                 | 0.012797775151119                                           | 1260               | $682 + 47n$                                               |
| 3-34 | $ee12 e34 e35 ee e55 e $                 | $11/54 - 16 \log[4/3]/27$                                   | 1260               | $628 + 100n + n^2$                                        |
| 3-35 | $ee12 e34 e35 e4 e5 ee $                 | 0.014252593468145                                           | 5040               | $674 + 55n$                                               |
| 3-36 | $ee12 345 345 ee ee ee $                 | 1/64                                                        | 52.5               | $672 + 54n + 3n^2$                                        |

Continued on next page

Table 1 Feynman graphs for effective coupling  $g_8$ 

| No.  | Graph description,<br>Nickel's notations | Integral value $\times (8\pi)^L$ ,<br>$L$ – number of loops | Symmetry<br>factor | Tensor factor $\times 3^{L+3}$ ,<br>$L$ – number of loops |
|------|------------------------------------------|-------------------------------------------------------------|--------------------|-----------------------------------------------------------|
| 4-1  | $ee11 22 33 45 ee6 ee6 ee $              | 1/8                                                         | 157.5              | $1264 + 656n + 232n^2 + 34n^3 + n^4$                      |
| 4-2  | $ee11 22 34 ee4 56 ee6 ee $              | 1/16                                                        | 315                | $1440 + 576n + 152n^2 + 18n^3 + n^4$                      |
| 4-3  | $ee11 22 34 ee5 ee5 66 ee $              | 1/8                                                         | 157.5              | $1392 + 624n + 152n^2 + 18n^3 + n^4$                      |
| 4-4  | $ee11 22 34 ee5 ee6 e66 e $              | 19/162                                                      | 315                | $1416 + 624n + 136n^2 + 11n^3$                            |
| 4-5  | $ee11 22 34 ee5 e56 e6 ee $              | 5/108                                                       | 1260               | $1512 + 552n + 116n^2 + 7n^3$                             |
| 4-6  | $ee11 22 34 ee5 e66 ee6 e $              | 19/162                                                      | 630                | $1416 + 624n + 136n^2 + 11n^3$                            |
| 4-7  | $ee11 22 34 ee5 566 ee ee $              | 1/8                                                         | 315                | $1392 + 624n + 152n^2 + 18n^3 + n^4$                      |
| 4-8  | $ee11 22 34 e45 e6 ee6 ee $              | 5/108                                                       | 630                | $1480 + 560n + 136n^2 + 11n^3$                            |
| 4-9  | $ee11 22 34 e56 e56 ee ee $              | 1/27                                                        | 315                | $1528 + 536n + 116n^2 + 7n^3$                             |
| 4-10 | $ee11 23 ee3 44 56 ee6 ee $              | 1/16                                                        | 315                | $1488 + 552n + 128n^2 + 18n^3 + n^4$                      |
| 4-11 | $ee11 23 ee3 45 ee5 66 ee $              | 1/16                                                        | 315                | $1520 + 544n + 108n^2 + 14n^3 + n^4$                      |
| 4-12 | $ee11 23 ee3 45 ee6 e66 e $              | 1/18                                                        | 1260               | $1576 + 532n + 74n^2 + 5n^3$                              |
| 4-13 | $ee11 23 ee3 45 e56 e6 ee $              | 1/36                                                        | 1260               | $1656 + 460n + 66n^2 + 5n^3$                              |
| 4-14 | $ee11 23 ee4 ee4 56 e66 e $              | 1/12                                                        | 315                | $1544 + 576n + 64n^2 + 3n^3$                              |
| 4-15 | $ee11 23 ee4 ee5 ee6 666  $              | $415/4608 - 5 \log[4/3]/16$                                 | 210                | $1272 + 816n + 96n^2 + 3n^3$                              |
| 4-16 | $ee11 23 ee4 ee5 e56 66 e $              | $-71/864 + 89 \log[4/3]/162$                                | 1260               | $1560 + 572n + 54n^2 + n^3$                               |
| 4-17 | $ee11 23 ee4 ee5 e66 e66  $              | 0.110545898524682                                           | 315                | $1424 + 624n + 130n^2 + 9n^3$                             |
| 4-18 | $ee11 23 ee4 ee5 556 6 ee $              | 31/384                                                      | 315                | $1544 + 576n + 64n^2 + 3n^3$                              |
| 4-19 | $ee11 23 ee4 e45 e5 66 ee $              | 5/108                                                       | 1260               | $1584 + 520n + 78n^2 + 5n^3$                              |
| 4-20 | $ee11 23 ee4 e45 e6 e66 e $              | $17/108 - 11 \log[4/3]/27$                                  | 2520               | $1640 + 500n + 46n^2 + n^3$                               |
| 4-21 | $ee11 23 ee4 e45 56 e6 ee $              | 19/864                                                      | 2520               | $1720 + 428n + 38n^2 + n^3$                               |
| 4-22 | $ee11 23 ee4 e45 66 ee6 e $              | $17/108 - 11 \log[4/3]/27$                                  | 1260               | $1624 + 504n + 56n^2 + 3n^3$                              |
| 4-23 | $ee11 23 ee4 e55 ee6 66 e $              | 0.110545898524682                                           | 630                | $1424 + 624n + 130n^2 + 9n^3$                             |
| 4-24 | $ee11 23 ee4 e55 e56 6 ee $              | $4 \log[4/3]/27$                                            | 1260               | $1600 + 516n + 68n^2 + 3n^3$                              |
| 4-25 | $ee11 23 ee4 e55 e66 e6 e $              | 0.110545898524682                                           | 1260               | $1520 + 588n + 76n^2 + 3n^3$                              |
| 4-26 | $ee11 23 ee4 e55 566 e ee $              | 19/162                                                      | 315                | $1504 + 592n + 86n^2 + 5n^3$                              |
| 4-27 | $ee11 23 ee4 e56 ee5 66 e $              | $-71/864 + 89 \log[4/3]/162$                                | 1260               | $1560 + 572n + 54n^2 + n^3$                               |
| 4-28 | $ee11 23 ee4 e56 e55 6 ee $              | $4 \log[4/3]/27$                                            | 1260               | $1600 + 516n + 68n^2 + 3n^3$                              |
| 4-29 | $ee11 23 ee4 e56 e56 e6 e $              | 0.019439866320025                                           | 2520               | $1744 + 414n + 29n^2$                                     |
| 4-30 | $ee11 23 ee4 e56 556 e ee $              | $-47/288 + 19 \log[4/3]/27$                                 | 1260               | $1640 + 500n + 46n^2 + n^3$                               |
| 4-31 | $ee11 23 ee4 445 6 ee6 ee $              | 13/256                                                      | 630                | $1592 + 528n + 64n^2 + 3n^3$                              |
| 4-32 | $ee11 23 ee4 455 e6 e6 ee $              | $17/108 - 11 \log[4/3]/27$                                  | 1260               | $1624 + 504n + 56n^2 + 3n^3$                              |
| 4-33 | $ee11 23 ee4 455 66 ee ee $              | 1/8                                                         | 157.5              | $1472 + 592n + 108n^2 + 14n^3 + n^4$                      |

Continued on next page

Table 1 Feynman graphs for effective coupling  $g_8$ 

| No.  | Graph description,<br>Nickel's notations | Integral value $\times (8\pi)^L$ ,<br>$L$ – number of loops | Symmetry<br>factor | Tensor factor $\times 3^{L+3}$ ,<br>$L$ – number of loops |
|------|------------------------------------------|-------------------------------------------------------------|--------------------|-----------------------------------------------------------|
| 4-34 | $ee11 23 ee4 456 ee e66 e $              | 1/12                                                        | 630                | $1544 + 576n + 64n^2 + 3n^3$                              |
| 4-35 | $ee11 23 ee4 456 e5 e6 ee $              | 19/864                                                      | 2520               | $1720 + 428n + 38n^2 + n^3$                               |
| 4-36 | $ee11 23 ee4 456 56 ee ee $              | 3/128                                                       | 630                | $1704 + 432n + 48n^2 + 3n^3$                              |
| 4-37 | $ee11 23 ee4 555 ee6 6 ee $              | $415/4608 - 5 \log[4/3]/16$                                 | 210                | $1272 + 816n + 96n^2 + 3n^3$                              |
| 4-38 | $ee11 23 ee4 556 ee5 6 ee $              | 31/384                                                      | 630                | $1544 + 576n + 64n^2 + 3n^3$                              |
| 4-39 | $ee11 23 ee4 556 ee6 e6 e $              | $-71/864 + 89 \log[4/3]/162$                                | 1260               | $1560 + 572n + 54n^2 + n^3$                               |
| 4-40 | $ee11 23 ee4 556 e56 e ee $              | $-47/288 + 19 \log[4/3]/27$                                 | 1260               | $1640 + 500n + 46n^2 + n^3$                               |
| 4-41 | $ee11 23 ee4 556 e66 ee e $              | 19/162                                                      | 630                | $1504 + 592n + 86n^2 + 5n^3$                              |
| 4-42 | $ee11 23 e34 e4 56 ee6 ee $              | 1/36                                                        | 630                | $1648 + 468n + 68n^2 + 3n^3$                              |
| 4-43 | $ee11 23 e34 e5 ee6 e66 e $              | $4 \log[4/3]/27$                                            | 2520               | $1608 + 512n + 64n^2 + 3n^3$                              |
| 4-44 | $ee11 23 e34 e5 e56 e6 ee $              | 1/54                                                        | 2520               | $1720 + 420n + 46n^2 + n^3$                               |
| 4-45 | $ee11 23 e34 45 e6 ee6 ee $              | 19/864                                                      | 2520               | $1688 + 444n + 54n^2 + n^3$                               |
| 4-46 | $ee11 23 e34 55 ee6 e6 ee $              | $4 \log[4/3]/27$                                            | 1260               | $1560 + 524n + 94n^2 + 9n^3$                              |
| 4-47 | $ee11 23 e34 56 ee5 e6 ee $              | 1/54                                                        | 2520               | $1704 + 424n + 56n^2 + 3n^3$                              |
| 4-48 | $ee11 23 e34 56 e56 ee ee $              | 7/432                                                       | 1260               | $1736 + 404n + 46n^2 + n^3$                               |
| 4-49 | $ee11 23 e44 e45 6 ee6 ee $              | $17/108 - 11 \log[4/3]/27$                                  | 1260               | $1616 + 512n + 58n^2 + n^3$                               |
| 4-50 | $ee11 23 e44 e55 e6 e6 ee $              | 0.110545898524682                                           | 630                | $1520 + 588n + 76n^2 + 3n^3$                              |
| 4-51 | $ee11 23 e44 e56 e5 e6 ee $              | $4 \log[4/3]/27$                                            | 2520               | $1632 + 504n + 50n^2 + n^3$                               |
| 4-52 | $ee11 23 e44 e56 56 ee ee $              | $11/54 - 16 \log[4/3]/27$                                   | 630                | $1648 + 488n + 50n^2 + n^3$                               |
| 4-53 | $ee11 23 e44 456 e ee6 ee $              | 1/18                                                        | 630                | $1584 + 532n + 68n^2 + 3n^3$                              |
| 4-54 | $ee11 23 e45 e45 ee 66 ee $              | 1/27                                                        | 315                | $1616 + 496n + 70n^2 + 5n^3$                              |
| 4-55 | $ee11 23 e45 e45 e6 e6 ee $              | 0.012797775151119                                           | 1260               | $1792 + 366n + 29n^2$                                     |
| 4-56 | $ee11 23 e45 e46 ee e66 e $              | $11/54 - 16 \log[4/3]/27$                                   | 1260               | $1656 + 484n + 46n^2 + n^3$                               |
| 4-57 | $ee11 23 e45 e46 e5 e6 ee $              | 0.014252593468146                                           | 5040               | $1776 + 382n + 29n^2$                                     |
| 4-58 | $ee11 23 e45 e46 56 ee ee $              | 1/54                                                        | 1260               | $1728 + 416n + 42n^2 + n^3$                               |
| 4-59 | $ee11 23 e45 446 e ee6 ee $              | $-47/288 + 19 \log[4/3]/27$                                 | 1260               | $1624 + 508n + 54n^2 + n^3$                               |
| 4-60 | $ee11 23 e45 456 ee e6 ee $              | 7/432                                                       | 2520               | $1752 + 396n + 38n^2 + n^3$                               |
| 4-61 | $ee11 23 e45 466 ee ee6 e $              | $11/54 - 16 \log[4/3]/27$                                   | 1260               | $1640 + 488n + 56n^2 + 3n^3$                              |
| 4-62 | $ee11 23 e45 466 e5 ee ee $              | 5/108                                                       | 630                | $1600 + 512n + 70n^2 + 5n^3$                              |
| 4-63 | $ee11 23 334 5 ee6 ee6 ee $              | 31/384                                                      | 315                | $1480 + 608n + 96n^2 + 3n^3$                              |
| 4-64 | $ee11 23 344 56 ee ee6 ee $              | 1/16                                                        | 157.5              | $1504 + 544n + 120n^2 + 18n^3 + n^4$                      |
| 4-65 | $ee11 23 345 46 ee ee6 ee $              | 3/128                                                       | 630                | $1672 + 448n + 64n^2 + 3n^3$                              |
| 4-66 | $ee11 23 456 456 ee ee ee $              | 1/64                                                        | 105                | $1752 + 384n + 48n^2 + 3n^3$                              |

Continued on next page

Table 1 Feynman graphs for effective coupling  $g_8$ 

| No.  | Graph description,<br>Nickel's notations | Integral value $\times (8\pi)^L$ ,<br>$L$ – number of loops  | Symmetry<br>factor | Tensor factor $\times 3^{L+3}$ ,<br>$L$ – number of loops |
|------|------------------------------------------|--------------------------------------------------------------|--------------------|-----------------------------------------------------------|
| 4-67 | $ee12 ee2 33 44 56 ee6 ee $              | 1/16                                                         | 78.75              | $1408 + 584n + 172n^2 + 22n^3 + n^4$                      |
| 4-68 | $ee12 ee2 33 45 ee6 e66 e $              | 1/18                                                         | 630                | $1560 + 540n + 82n^2 + 5n^3$                              |
| 4-69 | $ee12 ee2 33 45 e56 e6 ee $              | 1/36                                                         | 630                | $1624 + 476n + 82n^2 + 5n^3$                              |
| 4-70 | $ee12 ee2 34 ee4 56 e66 e $              | 1/24                                                         | 630                | $1616 + 516n + 52n^2 + 3n^3$                              |
| 4-71 | $ee12 ee2 34 ee5 ee6 666  $              | $125/3456 - \log[4/3]/8$                                     | 105                | $1344 + 780n + 60n^2 + 3n^3$                              |
| 4-72 | $ee12 ee2 34 ee5 e56 66 e $              | $-1/48 + 7 \log[4/3]/36$                                     | 1260               | $1656 + 500n + 30n^2 + n^3$                               |
| 4-73 | $ee12 ee2 34 ee5 e66 e66  $              | 0.050211596073066                                            | 630                | $1520 + 564n + 100n^2 + 3n^3$                             |
| 4-74 | $ee12 ee2 34 ee5 556 6 ee $              | 5/128                                                        | 630                | $1616 + 516n + 52n^2 + 3n^3$                              |
| 4-75 | $ee12 ee2 34 ee5 566 e6 e $              | $-1/48 + 7 \log[4/3]/36$                                     | 1260               | $1656 + 500n + 30n^2 + n^3$                               |
| 4-76 | $ee12 ee2 34 ee5 666 ee6  $              | $125/3456 - \log[4/3]/8$                                     | 210                | $1344 + 780n + 60n^2 + 3n^3$                              |
| 4-77 | $ee12 ee2 34 e45 e6 e66 e $              | $1/18 - \log[4/3]/9$                                         | 1260               | $1720 + 436n + 30n^2 + n^3$                               |
| 4-78 | $ee12 ee2 34 e45 56 e6 ee $              | 1/72                                                         | 2520               | $1784 + 372n + 30n^2 + n^3$                               |
| 4-79 | $ee12 ee2 34 e45 66 ee6 e $              | $1/18 - \log[4/3]/9$                                         | 1260               | $1680 + 452n + 52n^2 + 3n^3$                              |
| 4-80 | $ee12 ee2 34 e55 e56 6 ee $              | $1/18 - \log[4/3]/9$                                         | 1260               | $1688 + 452n + 46n^2 + n^3$                               |
| 4-81 | $ee12 ee2 34 e55 e66 e6 e $              | 0.050211596073066                                            | 630                | $1624 + 516n + 46n^2 + n^3$                               |
| 4-82 | $ee12 ee2 34 e56 e56 e6 e $              | 0.010868788166375                                            | 1260               | $1844 + 328n + 15n^2$                                     |
| 4-83 | $ee12 ee2 34 e56 556 e ee $              | $-1/24 + 2 \log[4/3]/9$                                      | 1260               | $1720 + 436n + 30n^2 + n^3$                               |
| 4-84 | $ee12 ee2 34 445 6 ee6 ee $              | 5/128                                                        | 315                | $1600 + 524n + 60n^2 + 3n^3$                              |
| 4-85 | $ee12 ee2 34 456 56 ee ee $              | 1/64                                                         | 315                | $1744 + 388n + 52n^2 + 3n^3$                              |
| 4-86 | $ee12 ee3 ee3 44 56 e66 e $              | 1/12                                                         | 315                | $1480 + 608n + 96n^2 + 3n^3$                              |
| 4-87 | $ee12 ee3 ee3 45 ee6 666  $              | $11/288 - \log[4/3]/8$                                       | 210                | $1272 + 816n + 96n^2 + 3n^3$                              |
| 4-88 | $ee12 ee3 ee3 45 e56 66 e $              | $\log[4/3]/6$                                                | 1260               | $1592 + 556n + 38n^2 + n^3$                               |
| 4-89 | $ee12 ee3 ee3 45 e66 e66  $              | 0.064928905166965                                            | 315                | $1488 + 608n + 90n^2 + n^3$                               |
| 4-90 | $ee12 ee3 ee3 45 556 6 ee $              | 1/16                                                         | 315                | $1480 + 608n + 96n^2 + 3n^3$                              |
| 4-91 | $ee12 ee3 ee4 ee5 566 66  $              | 0.000297739052128                                            | 315                | $1280 + 816n + 90n^2 + n^3$                               |
| 4-92 | $ee12 ee3 ee4 e45 e6 666  $              | $(-32321/540 - 577 \log[2] + 17 \log[3]/2 + 280 \log[5])/81$ | 420                | $1284 + 816n + 87n^2$                                     |
| 4-93 | $ee12 ee3 ee4 e45 56 66 e $              | 0.04307075173695                                             | 2520               | $1604 + 552n + 31n^2$                                     |
| 4-94 | $ee12 ee3 ee4 e45 66 e66  $              | 0.057786471957980                                            | 1260               | $1496 + 604n + 86n^2 + n^3$                               |
| 4-95 | $ee12 ee3 ee4 e55 e66 66  $              | 0.104584627154817                                            | 315                | $1288 + 656n + 216n^2 + 27n^3$                            |
| 4-96 | $ee12 ee3 ee4 e55 566 6 e $              | 0.071658392755453                                            | 1260               | $1500 + 604n + 83n^2$                                     |
| 4-97 | $ee12 ee3 ee4 e55 666 e6  $              | 0.000132225484595                                            | 420                | $1284 + 816n + 87n^2$                                     |
| 4-98 | $ee12 ee3 ee4 e56 e56 66  $              | 0.053569617411952                                            | 630                | $1500 + 604n + 83n^2$                                     |

Continued on next page

Table 1 Feynman graphs for effective coupling  $g_8$ 

| No.   | Graph description,<br>Nickel's notations | Integral value $\times (8\pi)^L$ ,<br>$L$ – number of loops   | Symmetry<br>factor | Tensor factor $\times 3^{L+3}$ ,<br>$L$ – number of loops |
|-------|------------------------------------------|---------------------------------------------------------------|--------------------|-----------------------------------------------------------|
| 4-99  | $ee12 ee3 ee4 e56 556 6 e $              | 0.042501325624530                                             | 2520               | $1604 + 552n + 31n^2$                                     |
| 4-100 | $ee12 ee3 ee4 445 6 e66 e $              | 0.062614832018137                                             | 630                | $1596 + 556n + 35n^2$                                     |
| 4-101 | $ee12 ee3 ee4 455 56 6 ee $              | 209/4608                                                      | 1260               | $1592 + 556n + 38n^2 + n^3$                               |
| 4-102 | $ee12 ee3 ee4 455 66 e6 e $              | 0.057786471957980                                             | 630                | $1600 + 552n + 34n^2 + n^3$                               |
| 4-103 | $ee12 ee3 ee4 456 56 e6 e $              | 0.020557711786                                                | 1260               | $1760 + 422n + 5n^2$                                      |
| 4-104 | $ee12 ee3 ee4 556 556  ee $              | $(-113 + 15\pi^2)/576$                                        | 315                | $1488 + 608n + 90n^2 + n^3$                               |
| 4-105 | $ee12 ee3 ee4 556 566 e e $              | 0.057602237765904                                             | 630                | $1604 + 552n + 31n^2$                                     |
| 4-106 | $ee12 ee3 e34 e4 56 e66 e $              | 5/162                                                         | 1260               | $1660 + 492n + 35n^2$                                     |
| 4-107 | $ee12 ee3 e34 e5 ee6 666  $              | $4909/11664 + 61 \log[2]/18$<br>$+ \log[3]/12 - 16 \log[5]/9$ | 840                | $1380 + 768n + 39n^2$                                     |
| 4-108 | $ee12 ee3 e34 e5 e56 66 e $              | 0.025133569519039                                             | 5040               | $1700 + 472n + 15n^2$                                     |
| 4-109 | $ee12 ee3 e34 e5 e66 e66  $              | 0.035640962304268                                             | 1260               | $1560 + 540n + 86n^2 + n^3$                               |
| 4-110 | $ee12 ee3 e34 e5 556 6 ee $              | 0.028534108723841                                             | 1260               | $1660 + 492n + 35n^2$                                     |
| 4-111 | $ee12 ee3 e34 45 e6 e66 e $              | 0.018537650414849                                             | 5040               | $1764 + 408n + 15n^2$                                     |
| 4-112 | $ee12 ee3 e34 45 56 e6 ee $              | 0.011176653628259                                             | 5040               | $1828 + 344n + 15n^2$                                     |
| 4-113 | $ee12 ee3 e34 45 66 ee6 e $              | 0.018537650414849                                             | 2520               | $1724 + 428n + 35n^2$                                     |
| 4-114 | $ee12 ee3 e34 55 ee6 66 e $              | 0.035640962304268                                             | 1260               | $1544 + 544n + 96n^2 + 3n^3$                              |
| 4-115 | $ee12 ee3 e34 55 e56 6 ee $              | $-65/1152 + 7 \log[4/3]/27$                                   | 2520               | $1720 + 428n + 38n^2 + n^3$                               |
| 4-116 | $ee12 ee3 e34 55 e66 e6 e $              | 0.035640962304268                                             | 2520               | $1656 + 492n + 38n^2 + n^3$                               |
| 4-117 | $ee12 ee3 e34 56 ee5 66 e $              | 0.025133569519039                                             | 2520               | $1692 + 476n + 19n^2$                                     |
| 4-118 | $ee12 ee3 e34 56 e55 6 ee $              | $-65/1152 + 7 \log[4/3]/27$                                   | 2520               | $1728 + 424n + 34n^2 + n^3$                               |
| 4-119 | $ee12 ee3 e34 56 e56 e6 e $              | 0.008397599554132                                             | 5040               | $1888 + 294n + 5n^2$                                      |
| 4-120 | $ee12 ee3 e34 56 556 e ee $              | 0.017290671286081                                             | 2520               | $1764 + 408n + 15n^2$                                     |
| 4-121 | $ee12 ee3 e44 e45 6 e66 e $              | 0.037085740379675                                             | 2520               | $1636 + 504n + 47n^2$                                     |
| 4-122 | $ee12 ee3 e44 e55 e6 66 e $              | 0.104584627154817                                             | 1260               | $1432 + 620n + 126n^2 + 9n^3$                             |
| 4-123 | $ee12 ee3 e44 e55 56 6 ee $              | 0.039515809496933                                             | 630                | $1568 + 520n + 90n^2 + 9n^3$                              |
| 4-124 | $ee12 ee3 e44 e56 e5 66 e $              | 0.071658392755453                                             | 2520               | $1572 + 568n + 47n^2$                                     |
| 4-125 | $ee12 ee3 e44 e56 55 6 ee $              | 0.039515809496933                                             | 1260               | $1496 + 556n + 126n^2 + 9n^3$                             |
| 4-126 | $ee12 ee3 e44 e56 56 e6 e $              | 0.018000831843930                                             | 2520               | $1712 + 430n + 45n^2$                                     |
| 4-127 | $ee12 ee3 e44 455 6 e6 ee $              | 0.037085740379675                                             | 1260               | $1628 + 508n + 51n^2$                                     |
| 4-128 | $ee12 ee3 e44 456 e e66 e $              | 19/243                                                        | 1260               | $1564 + 572n + 51n^2$                                     |
| 4-129 | $ee12 ee3 e44 456 5 e6 ee $              | 0.020141452226374                                             | 2520               | $1700 + 440n + 47n^2$                                     |
| 4-130 | $ee12 ee3 e44 555 e6 6 ee $              | 0.000132225484595                                             | 420                | $1284 + 816n + 87n^2$                                     |

Continued on next page

Table 1 Feynman graphs for effective coupling  $g_8$ 

| No.   | Graph description,<br>Nickel's notations | Integral value $\times (8\pi)^L$ ,<br>$L$ – number of loops | Symmetry<br>factor | Tensor factor $\times 3^{L+3}$ ,<br>$L$ – number of loops |
|-------|------------------------------------------|-------------------------------------------------------------|--------------------|-----------------------------------------------------------|
| 4-131 | $ee12 ee3 e44 556 e5 6 ee $              | 0.075942365596715                                           | 1260               | $1564 + 572n + 51n^2$                                     |
| 4-132 | $ee12 ee3 e44 556 e6 e6 e $              | 0.071658392755453                                           | 2520               | $1572 + 568n + 47n^2$                                     |
| 4-133 | $ee12 ee3 e44 556 56 e ee $              | 0.036300814059535                                           | 1260               | $1636 + 504n + 47n^2$                                     |
| 4-134 | $ee12 ee3 e45 e45 e6 66 e $              | 0.0152659449                                                | 2520               | $1776 + 398n + 13n^2$                                     |
| 4-135 | $ee12 ee3 e45 e45 56 6 ee $              | 0.011309549540615                                           | 1260               | $1808 + 350n + 29n^2$                                     |
| 4-136 | $ee12 ee3 e45 e46 ee 666  $              | 0.000233450823695                                           | 420                | $1380 + 768n + 39n^2$                                     |
| 4-137 | $ee12 ee3 e45 e46 e5 66 e $              | 0.015992626485276                                           | 5040               | $1744 + 414n + 29n^2$                                     |
| 4-138 | $ee12 ee3 e45 e46 55 6 ee $              | 0.025664756185216                                           | 2520               | $1668 + 488n + 31n^2$                                     |
| 4-139 | $ee12 ee3 e45 e46 56 e6 e $              | 0.009598391473892                                           | 5040               | $1850 + 327n + 10n^2$                                     |
| 4-140 | $ee12 ee3 e45 445 6 e6 ee $              | 0.016854227325864                                           | 2520               | $1764 + 408n + 15n^2$                                     |
| 4-141 | $ee12 ee3 e45 446 e e66 e $              | 0.034685049239056                                           | 2520               | $1668 + 488n + 31n^2$                                     |
| 4-142 | $ee12 ee3 e45 446 5 e6 ee $              | 0.017669745324596                                           | 2520               | $1732 + 424n + 31n^2$                                     |
| 4-143 | $ee12 ee3 e45 446 6 ee6 e $              | 0.024459585212457                                           | 2520               | $1692 + 476n + 19n^2$                                     |
| 4-144 | $ee12 ee3 e45 456 ee 66 e $              | 0.024251335395708                                           | 2520               | $1700 + 472n + 15n^2$                                     |
| 4-145 | $ee12 ee3 e45 456 e5 6 ee $              | 0.010445183225406                                           | 5040               | $1840 + 334n + 13n^2$                                     |
| 4-146 | $ee12 ee3 e45 456 e6 e6 e $              | 0.00803416337                                               | 5040               | $1898 + 287n + 2n^2$                                      |
| 4-147 | $ee12 ee3 e45 466 ee e66  $              | $121/576 + 17\pi^2/648$<br>$+ 38 Li_2[-1/3]/27$             | 1260               | $1560 + 540n + 86n^2 + n^3$                               |
| 4-148 | $ee12 ee3 e45 466 e5 e6 e $              | 0.015992626485276                                           | 5040               | $1776 + 398n + 13n^2$                                     |
| 4-149 | $ee12 ee3 e45 466 e6 ee6  $              | 0.023925239638591                                           | 2520               | $1700 + 472n + 15n^2$                                     |
| 4-150 | $ee12 ee3 e45 466 56 ee e $              | 0.027328814083503                                           | 2520               | $1668 + 488n + 31n^2$                                     |
| 4-151 | $ee12 ee3 e45 666 ee5 e6  $              | 0.000087219840724                                           | 840                | $1380 + 768n + 39n^2$                                     |
| 4-152 | $ee12 ee3 334 5 ee6 e66 e $              | 0.045781475051677                                           | 1260               | $1636 + 512n + 39n^2$                                     |
| 4-153 | $ee12 ee3 334 5 e56 e6 ee $              | 0.021734049853977                                           | 1260               | $1732 + 432n + 23n^2$                                     |
| 4-154 | $ee12 ee3 344 45 6 ee6 ee $              | 47/1536                                                     | 630                | $1664 + 496n + 26n^2 + n^3$                               |
| 4-155 | $ee12 ee3 344 55 e6 e6 ee $              | 0.035640962304268                                           | 630                | $1640 + 496n + 48n^2 + 3n^3$                              |
| 4-156 | $ee12 ee3 344 56 e5 e6 ee $              | $-65/1152 + 7 \log[4/3]/27$                                 | 2520               | $1752 + 412n + 22n^2 + n^3$                               |
| 4-157 | $ee12 ee3 344 56 56 ee ee $              | 7/384                                                       | 630                | $1744 + 416n + 26n^2 + n^3$                               |
| 4-158 | $ee12 ee3 345 45 e6 e6 ee $              | 0.009436905494                                              | 1260               | $1868 + 308n + 11n^2$                                     |
| 4-159 | $ee12 ee3 345 46 ee e66 e $              | 0.019629207404974                                           | 1260               | $1756 + 412n + 19n^2$                                     |
| 4-160 | $ee12 ee3 345 46 e5 e6 ee $              | 0.009209696800186                                           | 5040               | $1876 + 304n + 7n^2$                                      |
| 4-161 | $ee12 ee3 345 46 56 ee ee $              | 3/256                                                       | 1260               | $1816 + 348n + 22n^2 + n^3$                               |
| 4-162 | $ee12 ee3 445 446  ee6 ee $              | $(-145 + 18\pi^2)/768$                                      | 157.5              | $1536 + 560n + 90n^2 + n^3$                               |

Continued on next page

Table 1 Feynman graphs for effective coupling  $g_8$ 

| No.   | Graph description,<br>Nickel's notations | Integral value $\times (8\pi)^L$ ,<br>$L$ – number of loops   | Symmetry<br>factor | Tensor factor $\times 3^{L+3}$ ,<br>$L$ – number of loops |
|-------|------------------------------------------|---------------------------------------------------------------|--------------------|-----------------------------------------------------------|
| 4-163 | $ee12 ee3 445 456 e e6 ee $              | $-7/360 + 14 \log[2]/27$<br>$-161 \log[3]/864 - 7 \log[5]/96$ | 2520               | $1764 + 408n + 15n^2$                                     |
| 4-164 | $ee12 ee3 445 456 6 ee ee $              | $29/1536$                                                     | 1260               | $1720 + 428n + 38n^2 + n^3$                               |
| 4-165 | $ee12 ee3 445 466 e ee6 e $              | $0.034685049239056$                                           | 1260               | $1660 + 492n + 35n^2$                                     |
| 4-166 | $ee12 ee3 445 566 e6 ee e $              | $0.034058739909935$                                           | 630                | $1664 + 488n + 34n^2 + n^3$                               |
| 4-167 | $ee12 ee3 456 456 ee e6 e $              | $0.008764416908763$                                           | 1260               | $1888 + 294n + 5n^2$                                      |
| 4-168 | $ee12 e23 e3 45 ee6 e66 e $              | $2/81$                                                        | 2520               | $1716 + 440n + 31n^2$                                     |
| 4-169 | $ee12 e23 e3 45 e56 e6 ee $              | $1/81$                                                        | 1260               | $1804 + 356n + 27n^2$                                     |
| 4-170 | $ee12 e23 e4 ee4 56 e66 e $              | $5/162$                                                       | 2520               | $1676 + 484n + 27n^2$                                     |
| 4-171 | $ee12 e23 e4 ee5 ee6 666  $              | $0.000087219840724$                                           | 420                | $1380 + 768n + 39n^2$                                     |
| 4-172 | $ee12 e23 e4 ee5 e56 66 e $              | $0.027328814083503$                                           | 5040               | $1692 + 476n + 19n^2$                                     |
| 4-173 | $ee12 e23 e4 ee5 e66 e66  $              | $0.039515809496933$                                           | 2520               | $1544 + 544n + 96n^2 + 3n^3$                              |
| 4-174 | $ee12 e23 e4 ee5 556 6 ee $              | $0.029586081676179$                                           | 2520               | $1676 + 484n + 27n^2$                                     |
| 4-175 | $ee12 e23 e4 ee5 566 e6 e $              | $0.027328814083503$                                           | 5040               | $1692 + 476n + 19n^2$                                     |
| 4-176 | $ee12 e23 e4 e45 e6 e66 e $              | $0.015965685467107$                                           | 5040               | $1780 + 392n + 15n^2$                                     |
| 4-177 | $ee12 e23 e4 e45 56 e6 ee $              | $0.008957256127767$                                           | 10080              | $1868 + 308n + 11n^2$                                     |
| 4-178 | $ee12 e23 e4 e45 66 ee6 e $              | $0.015965685467107$                                           | 5040               | $1764 + 400n + 23n^2$                                     |
| 4-179 | $ee12 e23 e4 e55 e56 6 ee $              | $11/108 - 8 \log[4/3]/27$                                     | 5040               | $1736 + 412n + 38n^2 + n^3$                               |
| 4-180 | $ee12 e23 e4 e55 e66 e6 e $              | $0.039515809496933$                                           | 2520               | $1648 + 496n + 42n^2 + n^3$                               |
| 4-181 | $ee12 e23 e4 e56 e56 e6 e $              | $0.007617697226747$                                           | 5040               | $1892 + 288n + 7n^2$                                      |
| 4-182 | $ee12 e23 e4 e56 556 e ee $              | $0.015443212053930$                                           | 5040               | $1780 + 392n + 15n^2$                                     |
| 4-183 | $ee12 e23 e4 456 56 ee ee $              | $7/720$                                                       | 1260               | $1852 + 316n + 19n^2$                                     |
| 4-184 | $ee12 e23 34 e5 ee6 e66 e $              | $0.020141452226374$                                           | 5040               | $1748 + 416n + 23n^2$                                     |
| 4-185 | $ee12 e23 34 e5 e66 ee6 e $              | $0.020141452226374$                                           | 5040               | $1748 + 416n + 23n^2$                                     |
| 4-186 | $ee12 e23 34 56 ee5 e6 ee $              | $0.008957256127767$                                           | 5040               | $1852 + 316n + 19n^2$                                     |
| 4-187 | $ee12 e23 34 56 e56 ee ee $              | $0.008011413670392$                                           | 2520               | $1884 + 292n + 11n^2$                                     |
| 4-188 | $ee12 e23 44 ee5 e6 e66 e $              | $0.039515809496933$                                           | 2520               | $1616 + 508n + 60n^2 + 3n^3$                              |
| 4-189 | $ee12 e23 44 ee5 56 e6 ee $              | $11/108 - 8 \log[4/3]/27$                                     | 1260               | $1696 + 428n + 60n^2 + 3n^3$                              |
| 4-190 | $ee12 e23 44 e55 e6 e6 ee $              | $0.039515809496933$                                           | 2520               | $1616 + 508n + 60n^2 + 3n^3$                              |
| 4-191 | $ee12 e23 44 e56 56 ee ee $              | $-41/576 + 8 \log[4/3]/27$                                    | 1260               | $1752 + 396n + 38n^2 + n^3$                               |
| 4-192 | $ee12 e23 45 ee4 e6 e66 e $              | $0.015965685467107$                                           | 5040               | $1772 + 396n + 19n^2$                                     |
| 4-193 | $ee12 e23 45 ee4 66 ee6 e $              | $0.015965685467107$                                           | 2520               | $1756 + 404n + 27n^2$                                     |
| 4-194 | $ee12 e23 45 ee6 ee5 66 e $              | $11/108 - 8 \log[4/3]/27$                                     | 2520               | $1720 + 416n + 48n^2 + 3n^3$                              |

Continued on next page



Table 1 Feynman graphs for effective coupling  $g_8$ 

| No.   | Graph description,<br>Nickel's notations | Integral value $\times (8\pi)^L$ ,<br>$L$ – number of loops | Symmetry<br>factor | Tensor factor $\times 3^{L+3}$ ,<br>$L$ – number of loops |
|-------|------------------------------------------|-------------------------------------------------------------|--------------------|-----------------------------------------------------------|
| 4-195 | $ee12 e23 45 ee6 ee6 e66  $              | $(-3 + 16 \log[2] - 11 \log[3] + 3 \log[5])/54$             | 2520               | $1772 + 396n + 19n^2$                                     |
| 4-196 | $ee12 e23 45 ee6 e56 e6 e $              | 0.007617697226747                                           | 5040               | $1876 + 296n + 15n^2$                                     |
| 4-197 | $ee12 e23 45 e45 e6 e6 ee $              | 0.005830695492014                                           | 5040               | $1940 + 240n + 7n^2$                                      |
| 4-198 | $ee12 e23 45 e46 ee e66 e $              | 0.014318930502268                                           | 5040               | $1796 + 376n + 15n^2$                                     |
| 4-199 | $ee12 e23 45 e46 e5 e6 ee $              | 0.006284605628282                                           | 10080              | $1916 + 260n + 11n^2$                                     |
| 4-200 | $ee12 e23 45 e46 e6 ee6 e $              | 0.006284605628282                                           | 10080              | $1924 + 256n + 7n^2$                                      |
| 4-201 | $ee12 e23 45 e46 56 ee ee $              | 7/864                                                       | 2520               | $1864 + 300n + 22n^2 + n^3$                               |
| 4-202 | $ee12 e23 45 e66 ee5 e6 e $              | $11/108 - 8 \log[4/3]/27$                                   | 2520               | $1760 + 400n + 26n^2 + n^3$                               |
| 4-203 | $ee12 e23 45 e66 ee6 ee6  $              | $-41/576 + 8 \log[4/3]/27$                                  | 1260               | $1784 + 380n + 22n^2 + n^3$                               |
| 4-204 | $ee12 e23 45 456 ee e6 ee $              | 1/135                                                       | 2520               | $1900 + 276n + 11n^2$                                     |
| 4-205 | $ee12 e23 45 466 ee ee6 e $              | 0.014318930502268                                           | 2520               | $1780 + 384n + 23n^2$                                     |
| 4-206 | $ee12 e33 e34 5 ee6 e66 e $              | 0.037085740379675                                           | 2520               | $1652 + 496n + 39n^2$                                     |
| 4-207 | $ee12 e33 e34 5 e66 ee6 e $              | 0.037085740379675                                           | 2520               | $1652 + 496n + 39n^2$                                     |
| 4-208 | $ee12 e33 e44 e5 e6 e66 e $              | 0.104584627154817                                           | 1260               | $1528 + 584n + 72n^2 + 3n^3$                              |
| 4-209 | $ee12 e33 e44 e5 66 ee6 e $              | 0.104584627154817                                           | 630                | $1432 + 620n + 126n^2 + 9n^3$                             |
| 4-210 | $ee12 e33 e44 56 56 ee ee $              | 0.030132446707805                                           | 315                | $1656 + 480n + 48n^2 + 3n^3$                              |
| 4-211 | $ee12 e33 e45 e4 e6 e66 e $              | 0.037085740379675                                           | 5040               | $1660 + 492n + 35n^2$                                     |
| 4-212 | $ee12 e33 e45 e6 ee6 e66  $              | 0.036300814059535                                           | 2520               | $1660 + 492n + 35n^2$                                     |
| 4-213 | $ee12 e33 e45 e6 e55 6 ee $              | 0.071658392755453                                           | 2520               | $1572 + 568n + 47n^2$                                     |
| 4-214 | $ee12 e33 e45 e6 e56 e6 e $              | 0.018000831843930                                           | 5040               | $1760 + 406n + 21n^2$                                     |
| 4-215 | $ee12 e33 e45 45 e6 e6 ee $              | 0.011322590002467                                           | 2520               | $1808 + 358n + 21n^2$                                     |
| 4-216 | $ee12 e33 e45 46 ee e66 e $              | 0.029958025282025                                           | 2520               | $1676 + 476n + 35n^2$                                     |
| 4-217 | $ee12 e33 e45 46 e5 e6 ee $              | 0.012754884477300                                           | 5040               | $1792 + 374n + 21n^2$                                     |
| 4-218 | $ee12 e33 e45 46 e6 ee6 e $              | 0.012754884477300                                           | 5040               | $1768 + 386n + 33n^2$                                     |
| 4-219 | $ee12 e33 e45 66 ee6 ee6  $              | 0.030132446707805                                           | 630                | $1560 + 528n + 96n^2 + 3n^3$                              |
| 4-220 | $ee12 e33 345 e ee6 e66 e $              | 4/81                                                        | 1260               | $1628 + 516n + 43n^2$                                     |
| 4-221 | $ee12 e33 345 6 ee6 ee6 e $              | 0.013842067352976                                           | 1260               | $1780 + 384n + 23n^2$                                     |
| 4-222 | $ee12 e33 445 e6 e6 ee6 e $              | 0.036300814059535                                           | 2520               | $1660 + 492n + 35n^2$                                     |
| 4-223 | $ee12 e33 445 e6 56 ee ee $              | 0.075942365596715                                           | 630                | $1564 + 572n + 51n^2$                                     |
| 4-224 | $ee12 e33 445 56 e6 ee ee $              | 0.029958025282025                                           | 630                | $1668 + 480n + 39n^2$                                     |
| 4-225 | $ee12 e33 456 e4 ee e66 e $              | 19/243                                                      | 630                | $1564 + 572n + 51n^2$                                     |
| 4-226 | $ee12 e33 456 e4 56 ee ee $              | $5/288 + \log[5/3]/128$                                     | 1260               | $1740 + 420n + 27n^2$                                     |

Continued on next page

Table 1 Feynman graphs for effective coupling  $g_8$ 

| No.   | Graph description,<br>Nickel's notations | Integral value $\times (8\pi)^L$ ,<br>$L$ – number of loops | Symmetry<br>factor | Tensor factor $\times 3^{L+3}$ ,<br>$L$ – number of loops |
|-------|------------------------------------------|-------------------------------------------------------------|--------------------|-----------------------------------------------------------|
| 4-227 | $ee12 e34 e34 ee 56 e66 e $              | 2/81                                                        | 630                | $1700 + 464n + 23n^2$                                     |
| 4-228 | $ee12 e34 e34 e5 e6 e66 e $              | 0.011322590002467                                           | 2520               | $1832 + 346n + 9n^2$                                      |
| 4-229 | $ee12 e34 e34 56 56 ee ee $              | 0.005882277895645                                           | 630                | $1948 + 228n + 11n^2$                                     |
| 4-230 | $ee12 e34 e35 ee ee6 666  $              | $947/1458 + (148 \log[2] + 2 \log[3] - 76 \log[5])/27$      | 420                | $1404 + 756n + 27n^2$                                     |
| 4-231 | $ee12 e34 e35 ee e56 66 e $              | 0.021050665320974                                           | 2520               | $1724 + 452n + 11n^2$                                     |
| 4-232 | $ee12 e34 e35 ee e66 e66  $              | 0.030132446707805                                           | 630                | $1576 + 524n + 86n^2 + n^3$                               |
| 4-233 | $ee12 e34 e35 ee 556 6 ee $              | 0.023322339961950                                           | 630                | $1700 + 464n + 23n^2$                                     |
| 4-234 | $ee12 e34 e35 e4 e6 e66 e $              | 0.012754884477300                                           | 10080              | $1808 + 366n + 13n^2$                                     |
| 4-235 | $ee12 e34 e35 e6 ee5 66 e $              | 0.011756097196969                                           | 5040               | $1816 + 362n + 9n^2$                                      |
| 4-236 | $ee12 e34 e35 e6 ee6 e66  $              | 0.011888013318995                                           | 5040               | $1808 + 366n + 13n^2$                                     |
| 4-237 | $ee12 e34 e35 e6 e55 6 ee $              | 0.010929428448857                                           | 5040               | $1824 + 350n + 13n^2$                                     |
| 4-238 | $ee12 e34 e35 e6 e56 e6 e $              | 0.004660131730330                                           | 10080              | $1976 + 210n + n^2$                                       |
| 4-239 | $ee12 e34 e35 45 e6 e6 ee $              | 0.006349405102246                                           | 2520               | $1914 + 263n + 10n^2$                                     |
| 4-240 | $ee12 e34 e35 46 e5 e6 ee $              | 0.005585592314094                                           | 10080              | $1950 + 233n + 4n^2$                                      |
| 4-241 | $ee12 e34 e35 46 e6 ee6 e $              | 0.006847511971597                                           | 5040               | $1906 + 275n + 6n^2$                                      |
| 4-242 | $ee12 e34 e35 46 56 ee ee $              | 0.007643502650282                                           | 5040               | $1888 + 286n + 13n^2$                                     |
| 4-243 | $ee12 e34 e35 66 ee5 e6 e $              | 0.011756097196969                                           | 5040               | $1808 + 366n + 13n^2$                                     |
| 4-244 | $ee12 e34 e35 66 ee6 ee6  $              | 0.014486233305810                                           | 1260               | $1772 + 396n + 19n^2$                                     |
| 4-245 | $ee12 e34 e56 ee5 ee6 66  $              | 0.0204776278                                                | 1260               | $1716 + 456n + 15n^2$                                     |
| 4-246 | $ee12 e34 e56 ee5 e56 6 e $              | 0.006513602711906                                           | 10080              | $1918 + 265n + 4n^2$                                      |
| 4-247 | $ee12 e34 e56 ee5 e66 e6  $              | 0.012333968941018                                           | 2520               | $1776 + 382n + 29n^2$                                     |
| 4-248 | $ee12 e34 e56 ee5 556  ee $              | 0.014322122305123                                           | 1260               | $1780 + 392n + 15n^2$                                     |
| 4-249 | $ee12 e34 e56 e45 e6 e6 e $              | 0.005299982325608                                           | 5040               | $1948 + 236n + 3n^2$                                      |
| 4-250 | $ee12 e34 e56 e55 e66 e e $              | 0.029958025282025                                           | 1260               | $1684 + 472n + 31n^2$                                     |
| 4-251 | $ee12 e34 e56 e56 e56 e e $              | 0.004081559                                                 | 2520               | $2006 + 181n$                                             |
| 4-252 | $ee12 e34 335 6 e56 ee ee $              | 0.013026377750089                                           | 2520               | $1796 + 376n + 15n^2$                                     |
| 4-253 | $ee12 e34 345 ee e6 e66 e $              | 0.013842067352976                                           | 2520               | $1804 + 372n + 11n^2$                                     |
| 4-254 | $ee12 e34 345 e6 e6 ee6 e $              | 0.004971866553244                                           | 2520               | $1978 + 207n + 2n^2$                                      |
| 4-255 | $ee12 e34 345 e6 56 ee ee $              | 0.006413361170045                                           | 2520               | $1928 + 250n + 9n^2$                                      |
| 4-256 | $ee12 e34 355 ee e66 e6 e $              | 0.030132446707805                                           | 1260               | $1672 + 476n + 38n^2 + n^3$                               |
| 4-257 | $ee12 e34 356 ee ee5 66 e $              | 0.021050665320974                                           | 1260               | $1716 + 456n + 15n^2$                                     |
| 4-258 | $ee12 e34 356 ee e55 6 ee $              | $-41/576 + 8 \log[4/3]/27$                                  | 1260               | $1760 + 392n + 34n^2 + n^3$                               |

Continued on next page

Table 1 Feynman graphs for effective coupling  $g_8$ 

| No.   | Graph description,<br>Nickel's notations | Integral value $\times (8\pi)^L$ ,<br>$L$ – number of loops | Symmetry<br>factor | Tensor factor $\times 3^{L+3}$ ,<br>$L$ – number of loops |
|-------|------------------------------------------|-------------------------------------------------------------|--------------------|-----------------------------------------------------------|
| 4-259 | $ee12 e34 356 ee e56 e6 e $              | 0.006484168615633                                           | 2520               | $1920 + 262n + 5n^2$                                      |
| 4-260 | $ee12 e34 356 ee 556 e ee $              | 0.013220795118932                                           | 1260               | $1804 + 372n + 11n^2$                                     |
| 4-261 | $ee12 e34 356 e4 56 ee ee $              | 0.006108725710044                                           | 2520               | $1940 + 240n + 7n^2$                                      |
| 4-262 | $ee12 e34 356 e5 ee5 6 ee $              | 0.007466300196058                                           | 2520               | $1896 + 282n + 9n^2$                                      |
| 4-263 | $ee12 e34 356 e5 e56 e ee $              | 0.005298588893334                                           | 5040               | $1962 + 223n + 2n^2$                                      |
| 4-264 | $ee12 e34 356 45 e6 ee ee $              | 0.006922357564356                                           | 2520               | $1904 + 270n + 13n^2$                                     |
| 4-265 | $ee12 e34 556 e45 e6 e ee $              | 0.012333968941018                                           | 2520               | $1808 + 366n + 13n^2$                                     |
| 4-266 | $ee12 234 56 ee4 56 ee ee $              | 1/128                                                       | 630                | $1880 + 284n + 22n^2 + n^3$                               |
| 4-267 | $ee12 334 456 56 ee ee ee $              | 5/384                                                       | 157.5              | $1792 + 368n + 26n^2 + n^3$                               |
| 4-268 | $ee12 345 346 ee ee e66 e $              | 0.013555048885969                                           | 210                | $1812 + 360n + 15n^2$                                     |

Table 2: Feynman graphs for effective coupling  $g_{10}$ 

| No.                    | Graph description,<br>Nickel's notations | Integral value $\times (8\pi)^L$ ,<br>$L$ – number of loops | Symmetry<br>factor | Tensor factor $\times 3^{L+4}$ ,<br>$L$ – number of loops |
|------------------------|------------------------------------------|-------------------------------------------------------------|--------------------|-----------------------------------------------------------|
| 1-1                    | $ee12 ee3 ee4 ee4 ee $                   | 5/64                                                        | 11340              | $242 + n$                                                 |
| 2-1                    | $ee11 23 ee4 ee5 ee5 ee $                | 5/64                                                        | 28350              | $644 + 84n + n^2$                                         |
| 2-2                    | $ee12 ee2 34 ee5 ee5 ee $                | 1/32                                                        | 28350              | $692 + 36n + n^2$                                         |
| 2-3                    | $ee12 ee3 ee4 ee5 e55 e $                | 97/1296                                                     | 56700              | $646 + 83n$                                               |
| 2-4                    | $ee12 ee3 ee4 e45 e5 ee $                | 17/648                                                      | 113400             | $698 + 31n$                                               |
| 2-5                    | $ee12 ee3 e34 e5 ee5 ee $                | 1/48                                                        | 56700              | $710 + 19n$                                               |
| 2-6                    | $ee12 ee3 e45 e45 ee ee $                | 1/54                                                        | 56700              | $714 + 15n$                                               |
| 3-1                    | $ee11 22 34 ee5 ee6 ee6 ee $             | 5/64                                                        | 14175              | $1608 + 492n + 86n^2 + n^3$                               |
| 3-2                    | $ee11 23 ee3 45 ee6 ee6 ee $             | 1/32                                                        | 28350              | $1808 + 344n + 34n^2 + n^3$                               |
| 3-3                    | $ee11 23 ee4 ee4 56 ee6 ee $             | 1/32                                                        | 14175              | $1832 + 332n + 22n^2 + n^3$                               |
| 3-4                    | $ee11 23 ee4 ee5 ee5 66 ee $             | 5/64                                                        | 14175              | $1712 + 440n + 34n^2 + n^3$                               |
| 3-5                    | $ee11 23 ee4 ee5 ee6 e66 e $             | 97/1296                                                     | 56700              | $1720 + 438n + 29n^2$                                     |
| 3-6                    | $ee11 23 ee4 ee5 e56 e6 ee $             | 17/648                                                      | 56700              | $1856 + 318n + 13n^2$                                     |
| 3-7                    | $ee11 23 ee4 e45 e6 ee6 ee $             | 1/48                                                        | 113400             | $1880 + 294n + 13n^2$                                     |
| 3-8                    | $ee11 23 ee4 e55 ee6 e6 ee $             | 97/1296                                                     | 56700              | $1720 + 438n + 29n^2$                                     |
| 3-9                    | $ee11 23 ee4 e56 ee5 e6 ee $             | 17/648                                                      | 113400             | $1856 + 318n + 13n^2$                                     |
| 3-10                   | $ee11 23 ee4 e56 e56 ee ee $             | 1/54                                                        | 56700              | $1896 + 282n + 9n^2$                                      |
| 3-11                   | $ee11 23 ee4 456 ee ee6 ee $             | 1/32                                                        | 28350              | $1832 + 332n + 22n^2 + n^3$                               |
| 3-12                   | $ee11 23 ee4 556 ee6 ee ee $             | 5/64                                                        | 14175              | $1712 + 440n + 34n^2 + n^3$                               |
| 3-13                   | $ee11 23 e34 e5 ee6 ee6 ee $             | 17/648                                                      | 56700              | $1824 + 334n + 29n^2$                                     |
| 3-14                   | $ee11 23 e45 e46 ee ee6 ee $             | 1/54                                                        | 56700              | $1888 + 286n + 13n^2$                                     |
| 3-15                   | $ee12 ee2 33 45 ee6 ee6 ee $             | 1/32                                                        | 14175              | $1800 + 348n + 38n^2 + n^3$                               |
| 3-16                   | $ee12 ee2 34 ee4 56 ee6 ee $             | 1/64                                                        | 14175              | $1928 + 236n + 22n^2 + n^3$                               |
| 3-17                   | $ee12 ee2 34 ee5 ee6 e66 e $             | 19/648                                                      | 28350              | $1852 + 324n + 11n^2$                                     |
| 3-18                   | $ee12 ee2 34 ee5 e56 e6 ee $             | 5/432                                                       | 113400             | $1988 + 192n + 7n^2$                                      |
| 3-19                   | $ee12 ee2 34 ee5 e66 ee6 e $             | 19/648                                                      | 56700              | $1852 + 324n + 11n^2$                                     |
| 3-20                   | $ee12 ee2 34 e45 e6 ee6 ee $             | 5/432                                                       | 56700              | $1980 + 196n + 11n^2$                                     |
| 3-21                   | $ee12 ee2 34 e56 e56 ee ee $             | 1/108                                                       | 28350              | $2020 + 160n + 7n^2$                                      |
| 3-22                   | $ee12 ee3 ee3 45 ee6 e66 e $             | 1/36                                                        | 56700              | $1864 + 318n + 5n^2$                                      |
| 3-23                   | $ee12 ee3 ee3 45 e56 e6 ee $             | 1/72                                                        | 56700              | $1968 + 214n + 5n^2$                                      |
| Continued on next page |                                          |                                                             |                    |                                                           |

Table 2 Feynman graphs for effective coupling  $g_{10}$ 

| No.  | Graph description,<br>Nickel's notations | Integral value $\times (8\pi)^L$ ,<br>$L$ – number of loops | Symmetry<br>factor | Tensor factor $\times 3^{L+4}$ ,<br>$L$ – number of loops |
|------|------------------------------------------|-------------------------------------------------------------|--------------------|-----------------------------------------------------------|
| 3-24 | $ee12 ee3 ee4 ee4 56 e66 e $             | 5/96                                                        | 28350              | $1772 + 412n + 3n^2$                                      |
| 3-25 | $ee12 ee3 ee4 ee5 ee6 666  $             | $11609/184320 - 7 \log[4/3]/32$                             | 9450               | $1452 + 732n + 3n^2$                                      |
| 3-26 | $ee12 ee3 ee4 ee5 e56 66 e $             | $-1015/13824 + 551 \log[4/3]/1296$                          | 113400             | $1776 + 410n + n^2$                                       |
| 3-27 | $ee12 ee3 ee4 ee5 e66 e66  $             | 0.071839533099720                                           | 28350              | $1616 + 490n + 81n^2$                                     |
| 3-28 | $ee12 ee3 ee4 ee5 556 6 ee $             | 209/4096                                                    | 28350              | $1772 + 412n + 3n^2$                                      |
| 3-29 | $ee12 ee3 ee4 e45 e6 e66 e $             | $1021/7776 - 61 \log[4/3]/162$                              | 113400             | $1880 + 306n + n^2$                                       |
| 3-30 | $ee12 ee3 ee4 e45 56 e6 ee $             | 379/31104                                                   | 226800             | $1984 + 202n + n^2$                                       |
| 3-31 | $ee12 ee3 ee4 e45 66 ee6 e $             | $1021/7776 - 61 \log[4/3]/162$                              | 113400             | $1876 + 308n + 3n^2$                                      |
| 3-32 | $ee12 ee3 ee4 e55 e56 6 ee $             | $19/486 - 4 \log[4/3]/81$                                   | 113400             | $1828 + 332n + 27n^2$                                     |
| 3-33 | $ee12 ee3 ee4 e55 e66 e6 e $             | 0.071839533099720                                           | 56700              | $1724 + 436n + 27n^2$                                     |
| 3-34 | $ee12 ee3 ee4 e56 e56 e6 e $             | 0.011272671247075                                           | 113400             | $1990 + 197n$                                             |
| 3-35 | $ee12 ee3 ee4 e56 556 e ee $             | $-517/3456 + 97 \log[4/3]/162$                              | 113400             | $1880 + 306n + n^2$                                       |
| 3-36 | $ee12 ee3 ee4 445 6 ee6 ee $             | 163/6144                                                    | 28350              | $1868 + 316n + 3n^2$                                      |
| 3-37 | $ee12 ee3 ee4 456 56 ee ee $             | 13/1024                                                     | 28350              | $1980 + 204n + 3n^2$                                      |
| 3-38 | $ee12 ee3 e34 e5 ee6 e66 e $             | $-11/324 + 5 \log[4/3]/27$                                  | 226800             | $1900 + 284n + 3n^2$                                      |
| 3-39 | $ee12 ee3 e34 e5 e56 e6 ee $             | 7/864                                                       | 226800             | $2040 + 146n + n^2$                                       |
| 3-40 | $ee12 ee3 e34 45 e6 ee6 ee $             | 185/20736                                                   | 113400             | $2032 + 154n + n^2$                                       |
| 3-41 | $ee12 ee3 e34 55 ee6 e6 ee $             | $-11/324 + 5 \log[4/3]/27$                                  | 113400             | $1888 + 290n + 9n^2$                                      |
| 3-42 | $ee12 ee3 e34 56 ee5 e6 ee $             | 7/864                                                       | 226800             | $2036 + 148n + 3n^2$                                      |
| 3-43 | $ee12 ee3 e34 56 e56 ee ee $             | 71/10368                                                    | 113400             | $2072 + 114n + n^2$                                       |
| 3-44 | $ee12 ee3 e44 e55 e6 e6 ee $             | 0.071839533099720                                           | 56700              | $1724 + 436n + 27n^2$                                     |
| 3-45 | $ee12 ee3 e44 e56 e5 e6 ee $             | $19/486 - 4 \log[4/3]/81$                                   | 226800             | $1864 + 314n + 9n^2$                                      |
| 3-46 | $ee12 ee3 e44 e56 56 ee ee $             | $-11/162 + 8 \log[4/3]/27$                                  | 56700              | $1896 + 282n + 9n^2$                                      |
| 3-47 | $ee12 ee3 e45 e45 e6 e6 ee $             | 0.006047499233891                                           | 113400             | $2086 + 101n$                                             |
| 3-48 | $ee12 ee3 e45 e46 ee e66 e $             | $541/2592 - 2 \log[4/3]/3$                                  | 113400             | $1912 + 274n + n^2$                                       |
| 3-49 | $ee12 ee3 e45 e46 e5 e6 ee $             | 0.007043504786243                                           | 453600             | $2054 + 133n$                                             |
| 3-50 | $ee12 ee3 e45 e46 56 ee ee $             | 1/108                                                       | 113400             | $2000 + 178n + 9n^2$                                      |
| 3-51 | $ee12 ee3 e45 446 e ee6 ee $             | $-133/768 + 2 \log[4/3]/3$                                  | 56700              | $1904 + 282n + n^2$                                       |
| 3-52 | $ee12 ee3 e45 456 ee e6 ee $             | 79/10368                                                    | 226800             | $2048 + 138n + n^2$                                       |
| 3-53 | $ee12 ee3 e45 466 ee ee6 e $             | $541/2592 - 2 \log[4/3]/3$                                  | 113400             | $1908 + 276n + 3n^2$                                      |
| 3-54 | $ee12 ee3 345 46 ee ee6 ee $             | 19/2048                                                     | 28350              | $2028 + 156n + 3n^2$                                      |
| 3-55 | $ee12 ee3 456 456 ee ee ee $             | 7/1024                                                      | 9450               | $2076 + 108n + 3n^2$                                      |
| 3-56 | $ee12 e23 e4 ee5 ee6 e66 e $             | $541/2592 - 2 \log[4/3]/3$                                  | 113400             | $1864 + 314n + 9n^2$                                      |

Continued on next page

Table 2 Feynman graphs for effective coupling  $g_{10}$ 

| <b>No.</b> | <b>Graph description,<br/>Nickel's notations</b> | <b>Integral value <math>\times (8\pi)^L</math>,<br/><math>L</math> – number of loops</b> | <b>Symmetry<br/>factor</b> | <b>Tensor factor <math>\times 3^{L+4}</math>,<br/><math>L</math> – number of loops</b> |
|------------|--------------------------------------------------|------------------------------------------------------------------------------------------|----------------------------|----------------------------------------------------------------------------------------|
| 3-57       | $ee12 e23 e4 ee5 e56 e6 ee $                     | 1/108                                                                                    | 226800                     | $2012 + 172n + 3n^2$                                                                   |
| 3-58       | $ee12 e23 e4 e56 e56 ee ee $                     | 1/144                                                                                    | 113400                     | $2056 + 130n + n^2$                                                                    |
| 3-59       | $ee12 e23 45 ee6 ee6 ee6 e $                     | 1/144                                                                                    | 113400                     | $2052 + 132n + 3n^2$                                                                   |
| 3-60       | $ee12 e33 e45 e6 ee6 ee6 e $                     | $-11/162 + 8 \log[4/3]/27$                                                               | 113400                     | $1908 + 276n + 3n^2$                                                                   |
| 3-61       | $ee12 e34 e35 e6 ee5 e6 ee $                     | 0.005150554023338                                                                        | 226800                     | $2102 + 85n$                                                                           |
| 3-62       | $ee12 e34 e35 e6 ee6 ee6 e $                     | 0.005381671263319                                                                        | 75600                      | $2094 + 93n$                                                                           |
| 3-63       | $ee12 e34 e56 ee5 ee6 e6 e $                     | 0.006027278683541                                                                        | 75600                      | $2070 + 117n$                                                                          |
| 3-64       | $ee12 e34 356 ee e56 ee ee $                     | 29/5184                                                                                  | 28350                      | $2096 + 90n + n^2$                                                                     |
